# Supplementary material for: Informative Class Activation Maps
Source: arXiv:2106.10472 source file (2021-08-14)
Supplement: Supplementary file 1 [file appendix.tex]

%%%%%%%% ICML 2021 EXAMPLE LATEX SUBMISSION FILE %%%%%%%%%%%%%%%%%

\documentclass{article}

% Recommended, but optional, packages for figures and better typesetting:
\usepackage{microtype}
\usepackage{graphicx}
\usepackage{booktabs} % for professional tables

% ZQ packages
\usepackage{amsmath}
\usepackage{amsfonts}
\usepackage{multirow}
\usepackage{makecell}
\usepackage{rotating}

\usepackage{subcaption}
\usepackage[font=bf,labelfont=bf]{caption}

% hyperref makes hyperlinks in the resulting PDF.
% If your build breaks (sometimes temporarily if a hyperlink spans a page)
% please comment out the following usepackage line and replace
% \usepackage{icml2021} with \usepackage[nohyperref]{icml2021} above.
\usepackage{hyperref}

% ZQ commands 

% Attempt to make hyperref and algorithmic work together better:

% Use the following line for the initial blind version submitted for review:
% \usepackage{icml2021}

% If accepted, instead use the following line for the camera-ready submission:
\usepackage[accepted]{icml2021}

% The \icmltitle you define below is probably too long as a header.
% Therefore, a short form for the running title is supplied here:
\icmltitlerunning{
Supplementary Materials: 
Informative Class Activation Maps
}

\begin{document}

\twocolumn[
\icmltitle{Supplementary Materials: Informative Class Activation Maps 
}

\icmlsetsymbol{equal}{*}

\begin{icmlauthorlist}
\icmlauthor{Zhenyue Qin}{equal,anu}
\icmlauthor{Dongwoo Kim}{equal,anu,postech}
\icmlauthor{Tom Gedeon}{anu}
\end{icmlauthorlist}

\icmlaffiliation{anu}{School of Computing, Australian National University}
\icmlaffiliation{postech}{GSAI, PosTech, Korea}

\icmlcorrespondingauthor{Zhenyue Qin}{zhenyue.qin@anu.edu.au}
\icmlcorrespondingauthor{Dongwoo Kim}{dongwoo.kim@anu.edu.au}

% You may provide any keywords that you
% find helpful for describing your paper; these are used to populate
% the "keywords" metadata in the PDF but will not be shown in the document
% \icmlkeywords{Machine Learning, ICML}

\vskip 0.3in
]

% this must go after the closing bracket ] following \twocolumn[ ...

% This command actually creates the footnote in the first column
% listing the affiliations and the copyright notice.
% The command takes one argument, which is text to display at the start of the footnote.
% The \icmlEqualContribution command is standard text for equal contribution.
% Remove it (just {}) if you do not need this facility.

%\printAffiliationsAndNotice{}  % leave blank if no need to mention equal contribution

% Affiliations 
\printAffiliationsAndNotice{\icmlEqualContribution} % otherwise use the standard text.

\onecolumn
\input{secs/sup}

\newpage
% In the unusual situation where you want a paper to appear in the
% references without citing it in the main text, use \nocite
\nocite{langley00}

% \bibliography{refs}
% \bibliographystyle{icml2021}

\end{document}
